# Supplementary material for: Learning from Shader Program Traces
Source: arXiv:2102.04533 source file (2022-04-25)
Supplement: Supplementary file 1 [file supp_denoising_table.tex]

\vspace{-1ex}
\setlength{\tabcolsep}{2.0pt}
\begin{table}[]
\begin{tabular}{c|ccccc}
\hline

    \multirow{2}{*}{Shader} &  & \multicolumn{2}{c}{Perceptual} & \multicolumn{2}{c}{L2 Error} \\ \cline{3-6} 
    & Distances: & Similar & Different & Similar & Different \\ \thickhline

    \multicolumn{1}{c|}{\multirow{3}{*}{\begin{tabular}[c]{@{}c@{}}\bricks\\ Fig1 \end{tabular}}} & RGBx & 6.9e-03 & 2.3e-02 & 9.6e-05 & 2.1e-04 \\ \cline{2-6} 
    \multicolumn{1}{c|}{} & Ours & \textbf{28}\% & \textbf{23}\% & \textbf{36}\% & \textbf{28}\% \\ \cline{2-6}
    \multicolumn{1}{c|}{} & MSAA & 2760\% & 1044\% & 2354\% & 2011\% \\ \thickhline
    \multicolumn{1}{c|}{\multirow{3}{*}{\begin{tabular}[c]{@{}c@{}}\mandelbrot\\ Fig1 \end{tabular}}} & RGBx & 8.2e-03 & 9.2e-03 & 2.5e-04 & 2.3e-04 \\ \cline{2-6} 
    \multicolumn{1}{c|}{} & Ours & \textbf{40}\% & \textbf{46}\% & \textbf{54}\% & \textbf{64}\% \\ \cline{2-6}
    \multicolumn{1}{c|}{} & MSAA & 2460\% & 1890\% & 1238\% & 1129\% \\ \thickhline
    \multicolumn{1}{c|}{\multirow{3}{*}{\begin{tabular}[c]{@{}c@{}}\mandelbulb\\ Fig1 \end{tabular}}} & RGBx & 8.3e-03 & 9.5e-03 & 3.1e-04 & 2.7e-04 \\ \cline{2-6} 
    \multicolumn{1}{c|}{} & Ours & \textbf{64}\% & \textbf{64}\% & \textbf{65}\% & \textbf{70}\% \\ \cline{2-6}
    \multicolumn{1}{c|}{} & MSAA & 585\% & 627\% & 295\% & 362\% \\ \thickhline
    \multicolumn{1}{c|}{\multirow{3}{*}{\begin{tabular}[c]{@{}c@{}}\marble\\ Fig1 \end{tabular}}} & RGBx & 3.1e-02 & 4.4e-02 & 1.4e-03 & 1.7e-03 \\ \cline{2-6} 
    \multicolumn{1}{c|}{} & Ours & \textbf{61}\% & \textbf{61}\% & \textbf{53}\% & \textbf{50}\% \\ \cline{2-6}
    \multicolumn{1}{c|}{} & MSAA & 775\% & 660\% & 1231\% & 1389\% \\ \thickhline
    \multicolumn{1}{c|}{\multirow{3}{*}{\begin{tabular}[c]{@{}c@{}}\oceanic\\ Fig1 \end{tabular}}} & RGBx & 3.5e-02 & 4.1e-02 & 4.3e-04 & 4.4e-04 \\ \cline{2-6} 
    \multicolumn{1}{c|}{} & Ours & \textbf{83}\% & \textbf{79}\% & \textbf{78}\% & \textbf{81}\% \\ \cline{2-6}
    \multicolumn{1}{c|}{} & MSAA & 1190\% & 1111\% & 971\% & 1047\% \\ \thickhline
    \multicolumn{1}{c|}{\multirow{3}{*}{\begin{tabular}[c]{@{}c@{}}\primitives\\ Fig1 \end{tabular}}} & RGBx & 1.5e-02 & 1.3e-02 & 9.3e-05 & 8.3e-05 \\ \cline{2-6} 
    \multicolumn{1}{c|}{} & Ours & \textbf{75}\% & \textbf{72}\% & \textbf{89}\% & \textbf{85}\% \\ \cline{2-6}
    \multicolumn{1}{c|}{} & MSAA & 1725\% & 1821\% & 1781\% & 2041\% \\ \thickhline
    \multicolumn{1}{c|}{\multirow{3}{*}{\begin{tabular}[c]{@{}c@{}}\trippy\\ Fig1 \end{tabular}}} & RGBx & 7.3e-02 & 6.6e-02 & 2.4e-03 & 2.4e-03 \\ \cline{2-6} 
    \multicolumn{1}{c|}{} & Ours & \textbf{70}\% & \textbf{81}\% & \textbf{73}\% & \textbf{79}\% \\ \cline{2-6}
    \multicolumn{1}{c|}{} & MSAA & 316\% & 301\% & 254\% & 241\% \\ \thickhline
    \multicolumn{1}{c|}{\multirow{3}{*}{\begin{tabular}[c]{@{}c@{}}\venice\\ Fig1 \end{tabular}}} & RGBx & 3.1e-02 & 2.9e-02 & 6.0e-04 & 5.4e-04 \\ \cline{2-6} 
    \multicolumn{1}{c|}{} & Ours & \textbf{80}\% & \textbf{83}\% & \textbf{77}\% & \textbf{79}\% \\ \cline{2-6}
    \multicolumn{1}{c|}{} & MSAA & 921\% & 940\% & 754\% & 738\% \\ \hline
\end{tabular}
\caption{denoising}
\end{table}

\vspace{-1ex}
\setlength{\tabcolsep}{2.0pt}
\begin{table}[]
\begin{tabular}{c|ccccc}
\hline

    \multirow{2}{*}{Shader} &  & \multicolumn{2}{c}{Perceptual} & \multicolumn{2}{c}{L2 Error} \\ \cline{3-6} 
    & Distances: & Similar & Different & Similar & Different \\ \thickhline

\multicolumn{1}{c|}{\multirow{2}{*}{\begin{tabular}[c]{@{}c@{}}\bricks \end{tabular}}} & RGBx & 2.4e-02 & 4.9e-02 & 7.6e-04 & 8.3e-04 \\ \cline{2-6} 
    \multicolumn{1}{c|}{} & Ours & \textbf{37}\% & \textbf{41}\% & \textbf{29}\% & \textbf{53}\% \\ \thickhline
\multicolumn{1}{c|}{\multirow{2}{*}{\begin{tabular}[c]{@{}c@{}}\mandelbrot \end{tabular}}} & RGBx & 2.2e-01 & 2.9e-01 & 9.9e-03 & 1.7e-02 \\ \cline{2-6} 
    \multicolumn{1}{c|}{} & Ours & \textbf{23}\% & \textbf{17}\% & \textbf{24}\% & \textbf{10}\% \\ \thickhline
\multicolumn{1}{c|}{\multirow{2}{*}{\begin{tabular}[c]{@{}c@{}}\mandelbulb \end{tabular}}} & RGBx & 8.0e-02 & 5.3e-02 & 5.6e-03 & 2.5e-03 \\ \cline{2-6} 
    \multicolumn{1}{c|}{} & Ours & \textbf{56}\% & \textbf{43}\% & \textbf{59}\% & \textbf{43}\% \\ \thickhline
\multicolumn{1}{c|}{\multirow{2}{*}{\begin{tabular}[c]{@{}c@{}}\trippy \end{tabular}}} & RGBx & 2.2e-01 & 2.9e-01 & 1.3e-02 & 2.0e-02 \\ \cline{2-6} 
    \multicolumn{1}{c|}{} & Ours & \textbf{65}\% & \textbf{71}\% & \textbf{57}\% & \textbf{49}\% \\ \thickhline
\multicolumn{1}{c|}{\multirow{2}{*}{\begin{tabular}[c]{@{}c@{}}\venice \end{tabular}}} & RGBx & 4.3e-02 & 4.0e-02 & 9.3e-04 & 8.3e-04 \\ \cline{2-6} 
    \multicolumn{1}{c|}{} & Ours & \textbf{78}\% & \textbf{83}\% & \textbf{77}\% & \textbf{81}\% \\ \hline
\end{tabular}
\caption{simplified}
\end{table}

\vspace{-1ex}
\setlength{\tabcolsep}{2.0pt}
\begin{table}[]
\begin{tabular}{c|ccccc}
\hline

    \multirow{2}{*}{Shader} &  & \multicolumn{2}{c}{Perceptual} & \multicolumn{2}{c}{L2 Error} \\ \cline{3-6} 
    & Distances: & Similar & Different & Similar & Different \\ \thickhline

\multicolumn{1}{c|}{\multirow{2}{*}{\begin{tabular}[c]{@{}c@{}}\mandelbrot \end{tabular}}} & RGBx & 3.9e-03 & 6.4e-03 & 1.6e-04 & 1.7e-04 \\ \cline{2-6} 
    \multicolumn{1}{c|}{} & Ours & \textbf{81}\% & \textbf{73}\% & \textbf{72}\% & \textbf{85}\% \\ \thickhline
\multicolumn{1}{c|}{\multirow{2}{*}{\begin{tabular}[c]{@{}c@{}}\mandelbrot\\simplified \end{tabular}}} & RGBx & 1.7e-01 & 1.1e-01 & 1.2e-02 & 6.5e-03 \\ \cline{2-6} 
    \multicolumn{1}{c|}{} & Ours & \textbf{36}\% & \textbf{38}\% & \textbf{23}\% & \textbf{27}\% \\ \thickhline
\multicolumn{1}{c|}{\multirow{2}{*}{\begin{tabular}[c]{@{}c@{}}\mandelbulb \end{tabular}}} & RGBx & 8.0e-03 & 8.2e-03 & 3.2e-04 & 2.8e-04 \\ \cline{2-6} 
    \multicolumn{1}{c|}{} & Ours & \textbf{60}\% & \textbf{64}\% & \textbf{58}\% & \textbf{62}\% \\ \thickhline
\multicolumn{1}{c|}{\multirow{2}{*}{\begin{tabular}[c]{@{}c@{}}\mandelbulb\\simplified \end{tabular}}} & RGBx & 1.2e-01 & 7.4e-02 & 8.5e-03 & 4.4e-03 \\ \cline{2-6} 
    \multicolumn{1}{c|}{} & Ours & \textbf{62}\% & \textbf{57}\% & \textbf{52}\% & \textbf{45}\% \\ \thickhline
\multicolumn{1}{c|}{\multirow{2}{*}{\begin{tabular}[c]{@{}c@{}}\trippy\\simplified \end{tabular}}} & RGBx & 2.2e-01 & 3.1e-01 & 1.4e-02 & 2.6e-02 \\ \cline{2-6} 
    \multicolumn{1}{c|}{} & Ours & \textbf{59}\% & \textbf{63}\% & \textbf{46}\% & \textbf{49}\% \\ \hline
\end{tabular}
\caption{temporal}
\end{table}

\vspace{-1ex}
\setlength{\tabcolsep}{2.0pt}
\begin{table}[]
\begin{tabular}{c|ccccc}
\hline

    \multirow{2}{*}{Shader} &  & \multicolumn{2}{c}{Perceptual} & \multicolumn{2}{c}{L2 Error} \\ \cline{3-6} 
    & Distances: & Similar & Different & Similar & Different \\ \thickhline

\multicolumn{1}{c|}{\multirow{2}{*}{\begin{tabular}[c]{@{}c@{}}\mandelbulb\\blur \end{tabular}}} & RGBx & 6.3e-03 & 6.9e-03 & 2.3e-04 & 1.7e-04 \\ \cline{2-6} 
    \multicolumn{1}{c|}{} & Ours & \textbf{64}\% & \textbf{63}\% & \textbf{65}\% & \textbf{71}\% \\ \thickhline
\multicolumn{1}{c|}{\multirow{2}{*}{\begin{tabular}[c]{@{}c@{}}\trippy\\sharpen \end{tabular}}} & RGBx & 9.2e-02 & 8.6e-02 & 4.0e-03 & 3.8e-03 \\ \cline{2-6} 
    \multicolumn{1}{c|}{} & Ours & \textbf{69}\% & \textbf{82}\% & \textbf{70}\% & \textbf{80}\% \\ \thickhline
\multicolumn{1}{c|}{\multirow{2}{*}{\begin{tabular}[c]{@{}c@{}}\trippy\\simplified\ sharpen \end{tabular}}} & RGBx & 2.4e-01 & 3.1e-01 & 1.6e-02 & 2.5e-02 \\ \cline{2-6} 
    \multicolumn{1}{c|}{} & Ours & \textbf{74}\% & \textbf{80}\% & \textbf{62}\% & \textbf{57}\% \\ \hline
\end{tabular}
\caption{post\ processing}
\end{table}
